# Supplementary material for: Four-loop QCD MOM beta functions from the three-loop vertices at the symmetric point
Source: arXiv:2002.02875 ancillary file (2020-04-10)
Supplement: Supplementary file 1 [file info.pdf]

# Four-loop QCD MOM beta functions from the three-loop vertices at the symmetric point

A.Bednyakov, A.Pikelner

In the attached file `smom4l.m` we provide analytical answers for the following set of functions defined in the main article:

| <b>XCCG</b>      | <b>XQQG</b>      | <b>XGGG</b>      | <b>betaCCG</b>       | <b>betaQQG</b>       | <b>betaGGG</b>       |
|------------------|------------------|------------------|----------------------|----------------------|----------------------|
| $X_{\text{ccg}}$ | $X_{\text{qqg}}$ | $X_{\text{ggg}}$ | $\beta_{\text{ccg}}$ | $\beta_{\text{qqg}}$ | $\beta_{\text{ggg}}$ |

Results are presented for general color group in terms of the following symbols

|         | $N_A$     | $C_A$ | $C_F$              | $\frac{d_A^{abcd}d_A^{abcd}}{N_A}$ | $\frac{d_F^{abcd}d_A^{abcd}}{N_A}$ | $\frac{d_F^{abcd}d_F^{abcd}}{N_A}$ |
|---------|-----------|-------|--------------------|------------------------------------|------------------------------------|------------------------------------|
| code    | NA        | CA    | CF                 | dAA/NA                             | dFA/NA                             | dFF/NA                             |
| $SU(N)$ | $N^2 - 1$ | $N$   | $\frac{N^2-1}{2N}$ | $\frac{N^2(N^2+36)}{24}$           | $\frac{N(N^2+6)}{48}$              | $\frac{N^4-6N^2+18}{96N^2}$        |
| QCD     | 8         | 3     | 4/3                | 135/8                              | 15/16                              | 5/96                               |

and a set of constants defined in `Mathematica`:

| <b>pi</b> | <b>z3</b>  | <b>z5</b>  | <b>pg1</b>                | <b>pg3</b>                | <b>pg5</b>                |
|-----------|------------|------------|---------------------------|---------------------------|---------------------------|
| $\pi$     | $\zeta(3)$ | $\zeta(5)$ | $\psi^{(1)}(\frac{1}{3})$ | $\psi^{(3)}(\frac{1}{3})$ | $\psi^{(5)}(\frac{1}{3})$ |

In addition, we introduce two new constants **H5** and **H6** with uniform transcendental weight 5 and 6, respectively:

$$\mathbf{H5} = -23.931619569867810299556856128474147318843765098866$$

$$\mathbf{H6} = 248215.03828949457898954203375520678218766866096238$$

We provide two definitions for these constants and numerical values with precision of 6000 digits. The first one is in the file `subsHPL.m` and is written in terms of basis elements [1] consisting of the real parts of the harmonic polylogarithms at the argument  $e^{i\pi/3}$ . The second one (`subsGPL.m`) utilizes the basis of generalize polylogarithms at unity with indices  $r_{1,2} = e^{\pm i\pi/3}, r_{3,4} = e^{\pm 2i\pi/3}$ , constructed in [2].

For example, we evaluate numerically the coefficients of  $X_{\text{ccg}}$  for  $n_f = 4$ :

```

In[1]:= Get["smom4l.m"]; Get["subsHPL.m"];

In[2]:= colQCD = {CA → 3, CF → 4/3, TF → 1/2, NA → 8,
                  dAA → 135, dFA → 15/2, dFF → 5/12};

In[3]:= N[XCCG /. colQCD /. subsHPL /. nf → 4]

Out[3]= 1. + 14.1038 aMS + 319.469 aMS2 + 9173.2 aMS3

```

As another example, we evaluate numerically the coefficients of  $\beta_{\text{ccg}}$  for  $n_f = 4$ :

```

In[4]:= Get["smom4l.m"]; Get["subsHPL.m"];

In[5]:= colQCD = {CA → 3, CF → 4/3, TF → 1/2, NA → 8,
                  dAA → 135, dFA → 15/2, dFF → 5/12};

In[6]:= N[betaCCG /. colQCD /. subsHPL /. nf → 4]

Out[6]= -8.33333 accg2 - 51.3333 accg3 - 686.949 accg4 - 27900.5 accg5

```

The explicit form of the constant H5 in different bases:

$$\begin{aligned}
\text{H5} = & 7G_R(0, 0, 1; 1)G_I(r_2; 1)^2 + 27G_I(0, r_2; 1)G_I(0, 1, r_4; 1) \\
& - G_I(r_2; 1)^3G_I(0, r_2; 1) - 3G_I(r_2; 1)G_I(0, 0, 0, r_2; 1) \\
& + 18G_R(0, 0, 1, r_2, r_4; 1)
\end{aligned}$$

$$\begin{aligned}
\text{H5} = & 36\mathcal{R}_{-1,1,0,1,0} - \frac{6147}{5}\mathcal{R}_{-1,1,1,1,1} - 36\mathcal{R}_{1,-1,1,0,1} - 108\mathcal{R}_{1,-1,1,1,0} \\
& - \frac{849}{2}\mathcal{R}_{1,0,1,1,1} + \frac{40928}{435}\mathcal{R}_{1,1,-1,0,0} - \frac{87196}{435}\mathcal{R}_{1,1,-1,0,1} + 180\mathcal{R}_{1,1,1,0,-1} \\
& - \frac{118516}{435}\mathcal{R}_{1,1,-1,1,0} + \frac{175771}{145}\mathcal{R}_{1,1,-1,1,1} + 108\mathcal{R}_{1,1,0,1,-1} \\
& - \frac{167118683}{302760}\mathcal{R}_{1,1,0,1,1} - \frac{54880}{87}\mathcal{R}_{1,1,1,-1,0} + \frac{378946}{145}\mathcal{R}_{1,1,1,-1,1} \\
& - \frac{52745843}{181656}\mathcal{R}_{1,1,1,0,1} + \frac{22049}{5}\mathcal{R}_{1,1,1,1,-1} + \frac{191379739}{454140}\mathcal{R}_{1,1,1,1,0}
\end{aligned}$$

where we defined

$$\begin{aligned}
\mathcal{R}_{a_1, \dots, a_n} &= \text{Re} \left[ H_{a_1, \dots, a_n}(e^{i\pi/3}) \right] \\
G_R(a_1, \dots, a_n; 1) &= \text{Re} [G(a_1, \dots, a_n; 1)]
\end{aligned}$$

$$G_I(a_1, \dots, a_n; 1) = \text{Im} [G(a_1, \dots, a_n; 1)]$$

The explicit form of the constant H6 in different bases:

$$\begin{aligned} \text{H6} = & -95760G_I(r_2; 1)^3G_R(r_4; 1)G_I(0, r_2; 1) - 22680G_I(r_2; 1)^2G_R(0, 0, r_4, 1; 1) \\ & + 30240G_I(r_2; 1)G_R(r_4; 1)G_I(0, 0, 0, r_2; 1) + 48720G_R(0, 0, 1; 1)G_I(r_2; 1)G_I(0, r_2; 1) \\ & + 143640G_I(r_2; 1)^3G_I(0, 1, r_4; 1) + 147420G_I(r_2; 1)G_I(0, 0, 0, 1, r_4; 1) \\ & - 15120G_I(r_2; 1)^2G_I(0, r_2; 1)^2 + 226800G_I(r_2; 1)G_I(0, 0, 0, 1, r_2; 1) \\ & - 241920G_R(0, 0, 0, 0, r_2, r_4; 1) - 181440G_R(0, 0, 1, 1, r_4, r_2; 1) \\ & + 340200G_R(0, 0, 0, 0, r_4, 1; 1) + 119840G_R(0, 0, 1; 1)^2 \\ & - 90720G_I(r_2; 1)^4G_R(r_4; 1)^2 + 245277G_I(r_2; 1)^6 \end{aligned}$$

$$\begin{aligned} \text{H6} = & 362880\mathcal{R}_{-1,-1,1,0,1,0} - 12392352\mathcal{R}_{-1,-1,1,1,1,1} - 362880\mathcal{R}_{-1,1,-1,1,0,1} \\ & - 1088640\mathcal{R}_{-1,1,-1,1,1,0} - 4278960\mathcal{R}_{-1,1,0,1,1,1} + \frac{27503616}{29}\mathcal{R}_{-1,1,1,-1,0,0} \\ & - \frac{58595712}{29}\mathcal{R}_{-1,1,1,-1,0,1} - \frac{79642752}{29}\mathcal{R}_{-1,1,1,-1,1,0} + \frac{354354336}{29}\mathcal{R}_{-1,1,1,-1,1,1} \\ & + 1088640\mathcal{R}_{-1,1,1,0,1,-1} - \frac{5346908924}{841}\mathcal{R}_{-1,1,1,0,1,1} - \frac{184396800}{29}\mathcal{R}_{-1,1,1,1,-1,0} \\ & + \frac{763955136}{29}\mathcal{R}_{-1,1,1,1,-1,1} + 1814400\mathcal{R}_{-1,1,1,1,0,-1} - \frac{13392690220}{2523}\mathcal{R}_{-1,1,1,1,0,1} \\ & + 44450784\mathcal{R}_{-1,1,1,1,1,-1} + \frac{35892584}{2523}\mathcal{R}_{-1,1,1,1,1,0} - 362880\mathcal{R}_{1,-1,-1,1,0,1} \\ & - 1088640\mathcal{R}_{1,-1,-1,1,1,0} - \frac{40642560}{11}\mathcal{R}_{1,-1,1,-1,1,0} + \frac{182038752}{11}\mathcal{R}_{1,-1,1,-1,1,1} \\ & + 1088640\mathcal{R}_{1,-1,1,0,1,-1} + \frac{27216000}{11}\mathcal{R}_{1,-1,1,0,1,0} - \frac{1265440512}{319}\mathcal{R}_{1,-1,1,1,-1,0} \\ & + \frac{9113880384}{319}\mathcal{R}_{1,-1,1,1,-1,1} + 1814400\mathcal{R}_{1,-1,1,1,0,-1} + \frac{12167243424}{319}\mathcal{R}_{1,-1,1,1,1,-1} \\ & - \frac{7648252970708}{138765}\mathcal{R}_{1,-1,1,1,1,1} + \frac{27216000}{11}\mathcal{R}_{1,0,1,-1,1,0} - \frac{2762403840}{319}\mathcal{R}_{1,0,1,-1,1,1} \\ & - \frac{133912269610}{27753}\mathcal{R}_{1,0,1,0,1,1} + \frac{438484480}{319}\mathcal{R}_{1,0,1,1,-1,0} - \frac{3814742400}{319}\mathcal{R}_{1,0,1,1,-1,1} \\ & - \frac{448299133310}{83259}\mathcal{R}_{1,0,1,1,0,1} - \frac{3157015680}{319}\mathcal{R}_{1,0,1,1,1,-1} + \frac{395856568240}{83259}\mathcal{R}_{1,0,1,1,1,0} \\ & - \frac{73301760}{11}\mathcal{R}_{1,1,-1,-1,1,0} + \frac{263686752}{11}\mathcal{R}_{1,1,-1,-1,1,1} + 1088640\mathcal{R}_{1,1,-1,0,1,-1} \\ & - \frac{1147069056}{319}\mathcal{R}_{1,1,-1,1,-1,0} + \frac{10810820160}{319}\mathcal{R}_{1,1,-1,1,-1,1} + 1814400\mathcal{R}_{1,1,-1,1,0,-1} \\ & - \frac{146623580824}{27753}\mathcal{R}_{1,1,-1,1,0,1} + \frac{11141252640}{319}\mathcal{R}_{1,1,-1,1,1,-1} - \frac{566712413428}{27753}\mathcal{R}_{1,1,-1,1,1,0} \\ & + \frac{1188205660124}{138765}\mathcal{R}_{1,1,-1,1,1,1} + 1088640\mathcal{R}_{1,1,0,-1,1,-1} - \frac{4854349724}{841}\mathcal{R}_{1,1,0,-1,1,1} \end{aligned}$$

$$\begin{aligned}
& +1088640\mathcal{R}_{1,1,0,1,-1,-1} + \frac{1133838696249132812}{6295629285}\mathcal{R}_{1,1,0,1,-1,0} \\
& - \frac{465193321021842244}{2098543095}\mathcal{R}_{1,1,0,1,-1,1} - \frac{697902426440420612}{2098543095}\mathcal{R}_{1,1,0,1,1,-1} \\
& - \frac{389220277666736942}{2098543095}\mathcal{R}_{1,1,1,-1,-1,0} + \frac{466985281238385902}{2098543095}\mathcal{R}_{1,1,1,-1,-1,1} \\
& - \frac{46953057648}{4205}\mathcal{R}_{1,1,1,-1,0,-1} + \frac{14165415833633862}{233171455}\mathcal{R}_{1,1,1,-1,0,0} \\
& - \frac{859144693394712326}{6295629285}\mathcal{R}_{1,1,1,-1,0,1} + \frac{451246220656615502}{2098543095}\mathcal{R}_{1,1,1,-1,1,-1} \\
& - \frac{342700632118743586}{6295629285}\mathcal{R}_{1,1,1,-1,1,0} + \frac{467663616245334274}{2098543095}\mathcal{R}_{1,1,1,-1,1,1} \\
& +1814400\mathcal{R}_{1,1,1,0,-1,-1} + \frac{1435962426048582968}{2098543095}\mathcal{R}_{1,1,1,0,-1,0} \\
& - \frac{543182821801440296}{699514365}\mathcal{R}_{1,1,1,0,-1,1} + \frac{167187424712}{2523}\mathcal{R}_{1,1,1,0,0,-1} \\
& + \frac{552441908228400766}{11332132713}\mathcal{R}_{1,1,1,0,0,1} - \frac{260072928578724088}{233171455}\mathcal{R}_{1,1,1,0,1,-1} \\
& - \frac{2211248256225309688}{56660663565}\mathcal{R}_{1,1,1,0,1,0} + \frac{1592115366408910808}{2098543095}\mathcal{R}_{1,1,1,1,-1,-1} \\
& + \frac{419428930312070258}{2098543095}\mathcal{R}_{1,1,1,1,-1,0} + \frac{938578319363231702}{2098543095}\mathcal{R}_{1,1,1,1,-1,1} \\
& - \frac{64337983979177944}{24121185}\mathcal{R}_{1,1,1,1,0,-1} + \frac{1937948230299237521}{50365034280}\mathcal{R}_{1,1,1,1,0,0} \\
& + \frac{51618028314896914}{139902873}\mathcal{R}_{1,1,1,1,1,-1} - \frac{14051838957873018177019}{288454287240}\mathcal{R}_{1,1,1,1,1,1}
\end{aligned}$$

## References

- [1] B. A. Kniehl, A. F. Pikelner, and O. L. Veretin. Three-loop massive tadpoles and polylogarithms through weight six. *JHEP*, 08:024, 2017.
- [2] Johannes M. Henn, Alexander V. Smirnov, and Vladimir A. Smirnov. Evaluating Multiple Polylogarithm Values at Sixth Roots of Unity up to Weight Six. *Nucl. Phys.*, B919:315–324, 2017.
